# Supplementary material for: Coexistence of Superconductivity and Antiferromagnetism in the Hubbard model for cuprates
Source: arXiv:1811.12363 source file (2019-06-19)
Supplement: Supplementary file 1 [file suppl_material.pdf]

# Supplementary material for
## *Coexistence of Superconductivity and Antiferromagnetism in the Hubbard model for cuprates*

A. Foley,[1] S. Verret,[1] A.-M. S. Tremblay,[1,2] and D. Sénéchal[1]

[1]*Département de physique and Institut quantique, Université de Sherbrooke, Sherbrooke, Québec, Canada J1K 2R1*
[2]*Canadian Institute for Advanced Research, Toronto, Ontario, Canada, M5G 1Z8*

(Dated: November 28, 2018)

### I. DIFFERENCES BETWEEN CLUSTER AND LATTICE AVERAGES

In this section we will comment on the differences that arise between lattice averages and cluster averages, as explained in Sect. IID of the paper. Figure A shows the order parameters as a function of density for YBCO parameters, the equivalent of Fig. 3 of the paper, except that all quantities (order parameters and density) are *cluster* averages. Recall that in the main text, averages of local operators (density and staggered magnetization) are *cluster averages*, and averages of bond operators ($\hat{D}$ and $\hat{\pi}$) are *lattice averages*. When comparing with Fig. 3 of the paper, only the latter should differ. Indeed, we find that the $d$SC order parameter is slightly enhanced when using lattice averages. Curiously, the $\pi$-triplet order parameter is much enhanced when using lattice averages, but only in the general parametrization.

Figure C shows similar data, this time for the NCCO system, and therefore should be compared to Fig. 4 of the paper. Again, using lattice averages enhances the $d$SC order parameter, but comparing different averages of the $\pi$-triplet order parameter is trickier: the latter is sometimes enhanced by using lattice averages, sometimes not. However, the behavior of the cluster-averaged $d$SC order parameter is pathological: on the upper panel ($U = 5$), it is sometimes larger in the coexistence solution than in the pure $d$SC solution, as if it were cooperating rather than competing with antiferromagnetism. This is not observed when considering lattice averages for the nonlocal operators and leads us to think that the latter are preferable when dealing with nonlocal operators.

Figure B shows the order parameters as a function of density for YBCO parameters, the equivalent of Fig. 3 of the paper, except that all quantities (order parameters and density) are *lattice* averages. The comparison is more difficult, because the horizontal axis is not the same, but the values of the nonlocal order parameters should be the same as on Fig. 3 of the paper. The difference between these curves and Fig. 3 are minor. The cluster density extends a bit further both on the hole- and electron-doped sides.

Finally, Fig. D for the NCCO parameters is computed with lattice averages, and should again be compared to Fig. 4 of the paper. There, important differences appear at $U = 5$: the lattice density extends far less than the cluster density, is even shows re-entrant behavior on the edge of the pure $d$SC phase on the hole-doped side, which is clearly defective. In addition, the pure $d$SC phase and the microscopic coexistence phase overlap in density, which makes no sense thermodynamically and can only be attributed to an erroneous estimation of the density. Things are much better at $U = 6.55$, which makes us think that the main disagreement between the different averages are amplified below the Mott transition.

Overall, these differences, especially in the $U = 5$ case for NCCO, convince us that the best strategy is to use cluster averages for local operators and lattice averages for nonlocal ones.

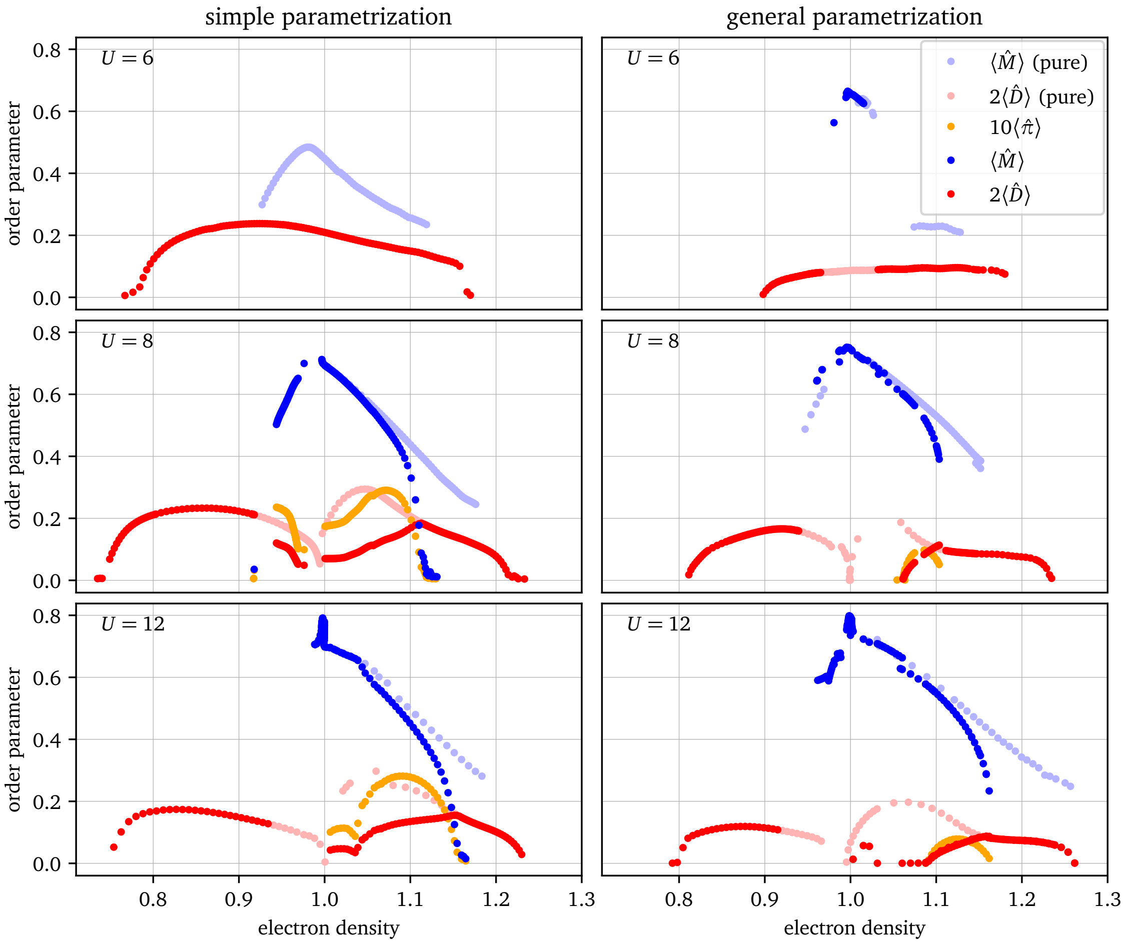


Figure A. Order parameters as a function of density for YBCO parameters. The same description as Fig. 3 of the main paper applies, except that all quantities (order parameters and electron density) are **cluster** averages.

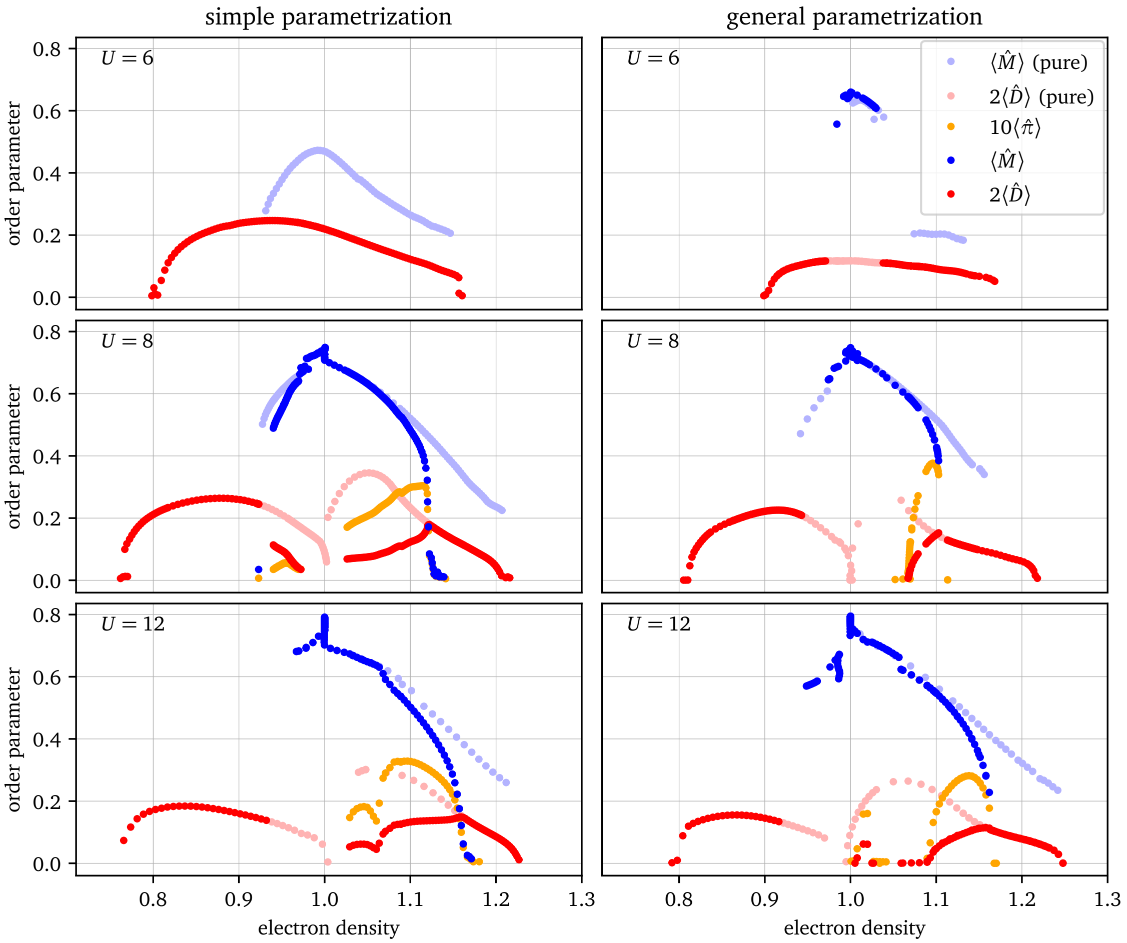


Figure B. Order parameters as a function of density for YBCO parameters. The same description as Fig. 3 of the main paper applies, except that all quantities (order parameters and electron density) are **lattice** averages.

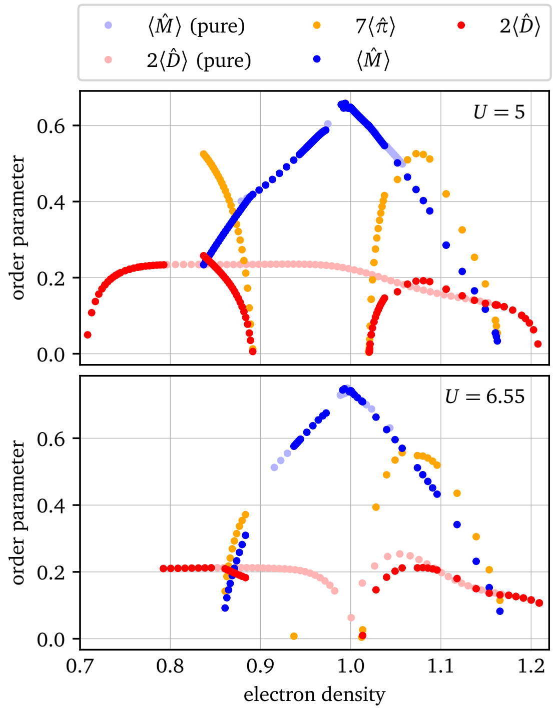


Figure C. Order parameters as a function of density for NCCO parameters. The same description as Fig. 4 of the main paper applies, except that all quantities (order parameters and electron density) are **cluster** averages.

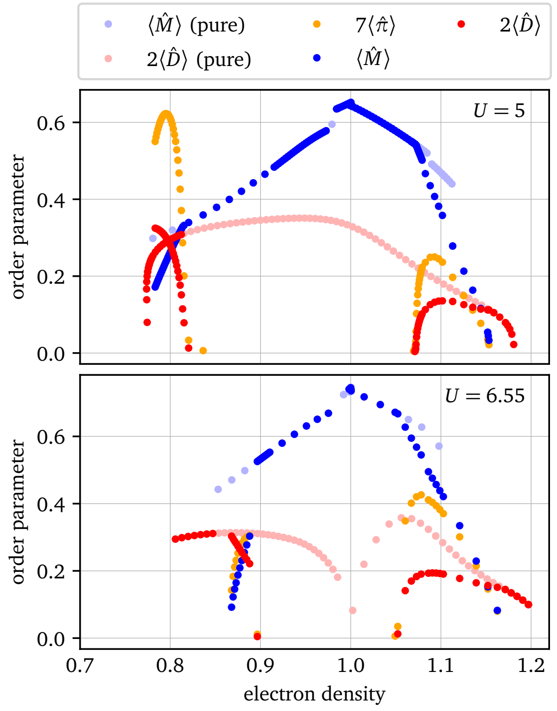


Figure D. Order parameters as a function of density for NCCO parameters. The same description as Fig. 4 of the main paper applies, except that all quantities (order parameters and electron density) are **lattice** averages.
